# Supplementary material for: $D$-modules arithm\'etiques, distributions et localisation
Source: arXiv:1401.6901 source file (2017-06-26)
Supplement: Supplementary file 1 [file appendice.tex]

\appendix
%ajoute une ligne appendice
%\addcontentsline{toc}{section}{Appendice : Opérateurs différentiels
%arithmétiques globaux sur les variétés de drapeaux (par Christine Huyghe)}
%supprime l'affichage des sections dans la toc, section correspond a 0
%\addtocontents{toc}{\protect\setcounter{tocdepth}{0}}
%\addtocontents{toc}{\protect\setcounter{tocdepth}{2}}
\section[Appendice : calculs de sections globales (par Christine Huyghe)]{Appendice : Opérateurs différentiels
arithmétiques globaux sur les variétés de drapeaux (par Christine Huyghe)}
\subsection{Introduction}
Nous nous plaçons ici dans le cas où $V$ est un anneau de valuation discrètes d'inégales caractéristiques ($0$,$p$),
$S=\spec V$,
et reprenons les notations de ~\ref{section-rappels}. Nous supposons de plus que $G$ est  
un schéma en groupes réductif $G$, connexe, déployé sur $S$. On note
 $X$ la variété de drapeaux de $G$, $\GG$
(resp. $\XX$) la variété de 
drapeaux formelle obtenue en complétant $p$-adiquement $G$ (resp. $\XX$) le long de l'idéal $\pi$.
Soit $T$ un tore maximal de $G$, et $\lam$ un caractère de $T$ qui est un poids dominant et régulier. Ceci est équivalent 
à dire que le faisceau inversible $G$-équivariant sur la variété de drapeaux $X$, $\LL(\lam)$, qui est associé
à $\lam$ par la construction habituelle, est ample et vérifie $\Ga(X,\LL(\lam))\neq 0$. 

On note $\TT_X$ le faisceau tangent sur $X$, $\DD_X$ le faisceau usuel des opérateurs 
différentiels construit dans \cite{EGA4-4}, $\DD^{(m)}_{X}$, $\Dcm_{\XX}$ les faisceaux 
introduits en~\ref{operateur-diff}.

Nous utiliserons aussi les algèbres de distributions $D^{(m)}(G)$, $\what{D}^{(m)}(\GG)$, et 
$D^{\dagger}(\GG)_{\Qr}$ introduites en~\ref{sect-distribution-algebras}. L'algèbre opposée 
d'une algèbre $U$ sera notée $U^{op}$.

\subsection[Opérateurs différentiels sur la variété de drapeaux]{Sections globales des opérateurs différentiels arithmétiques sur la variété de drapeaux}
\label{rappels-Uclass}
%
\subsubsection{Rappels du cas classique}
%}
On considère ici le groupe $G_K=G\times_S \spec K$, $X_K$ la variété de drapeaux de 
$G_K$, obtenue par changement de base à partir de $X$.

Soient $U_K=U(Lie(G_K))$ l'algèbre enveloppante de $Lie(G_K)$, 
$Z_K$ son centre et 
$\xi_1,\ldots,\xi_N$ une base de $Lie(G)$. On se donne un plongement 
$\iota$ : $K \rig \Cc$. On peut alors considérer le groupe $G_{\Cc}$, 
$X_{\Cc}$ la variété de drapeaux et $Lie(G_{\Cc})= Lie(G)\ot_K \Cc$. 
De ce fait, l'algèbre enveloppante notée $U_{\Cc}$ de $Lie(G_{\Cc})$ 
est isomorphe à $\Cc\ot_K U_K$. Soit $Z_{\Cc}$ son centre. Si $a\in U_K$, on note 
$$\xymatrix @R=0mm {C_a \colon & U_K \ar@{->}[r] & U_K \\
                     & x \ar@{{|}->}[r] & [a,x].}$$ 
On vérifie alors facilement que $Z_K=\bigcap_{i=1}^N Ker(C_{\xi_i})$, ce qui 
montre que $Z_{\Cc}= \Cc \ot_K Z_K$. De même, si on note 
${Z_{K}}_+=Z_K\bigcap Lie(G)U_K$ (resp. ${Z_{\Cc}}_+=Z_{\Cc}\bigcap Lie(G)U_{\Cc}$), 
alors ${Z_{\Cc}}_+= \Cc\ot_K {Z_{K}}_+$. 

De plus, $\DD_{X_{\Cc}}=\Cc\ot_K \DD_{X_{K}}$, de sorte que 
$\Ga(X_{\Cc},\DD_{\XX_{\Cc}})=\Cc\ot_K \Ga(X_K,\DD_{X_{K}})$. En particulier 
on dispose d'injections canoniques 
$$\xymatrix @R=0mm {j_D \colon & \Ga(X_K,\DD_{X_K})\ar@{^{(}->}[r]& \Ga(X_{\Cc},\DD_{X_{\Cc}})\\
                   & x \ar@{{|}->}[r] & 1\ot x}$$
resp. $j_U$ : $U_K \hrig U_{\Cc}$. Comme en ~\ref{op_diff_inv}, l'action de $G$ sur $X$ 
induit un antihomomorphisme $Q_K$ : $U_K \rig \Ga(X_K,\DD_{X_K})$ (resp. 
$Q_{\Cc}=1\ot Q_K$ : $U_{\Cc} \rig \Ga(X_{\Cc},\DD_{X_{\Cc}})$).  
Il résulte de~\cite{BeBe} que $Q_{\Cc}({Z_{\Cc}}_+)=0$ et que l'on a un isomorphisme de $\Cc$-algèbres
$$ Q_{\Cc} \,\colon \, U_{\Cc}^{op}/{Z_{\Cc}}_+ \sta{\sim}{\rig} \Ga(X_{\Cc},\DD_{X_{\Cc}}).$$
 Ceci implique que $Q_K({Z_{K}}_+)=0$ et que l'on a un isomorphisme de $K$-algèbres
$$ Q_{K} \,\colon \, U_K^{op}/{Z_{K}}_+ \sta{\sim}{\rig} \Ga(X_{K},\DD_{X_{K}}).$$

Dans le cas twisté, la situation est la suivante. Soient $\lam$ un poids dominant et régulier de $T$, $\LL(\lam)$ le 
faisceau inversible associé sur $X$. D'après~\ref{Qtmc}, on dispose d'un antihomomorphisme 
$^t{}Q_K$ : $U_K^{op} \rig \Ga(X_K,^t{}\DD_{X_K})$, où $^t{}\DD_{X_K}=\LL(\lam)\ot_{\OO_X}\DD_{X_K}\ot_{\OO_X}\LL(\lam)^{-1}$.
Alors, toujours d'après~\cite{BeBe}, $^t{}Q(Z_{\Cc})\subset \Cc$, de sorte que $^t{}Q(Z_{K})\subset K$, ce qui définit  
un caractère $\theta$ : $Z_K \rig K$. Alors, 
par loc. cit., $^t{}Q_{\Cc}$ induit un isomorphisme
  $$ ^t{}Q_{\Cc} \,\colon \, U_{\Cc}^{op}/Ker\theta_{\Cc} U_{\Cc}^{op}\sta{\sim}{\rig} \Ga(X_{\Cc},^t{}\DD_{X_{\Cc}}).$$
Les mêmes arguments que précédemment montrent que cet isomorphisme se descend en un isomorphisme de $K$-algèbres
$$ ^t{}Q_{K} \,\colon \, U_K^{op}/ Ker\theta_K \, U_{K}^{op}\sta{\sim}{\rig} \Ga(X_{K},\DD_{X_{K}}).$$
%
%\subsubsection{Opérateurs différentiels tordus sur la variété de drapeaux}
%
%On suppose dans ce cas que $G$ est déployé sur $S$...
%
\subsubsection{Enoncé du théorème}
\label{enonce-thm_class}
%
Soit $m\in\Ne$, on dispose de l'application $Q_m$ introduite en ~\ref{def_Qmc}, 
$Q_m $ : $\what{D}^{(m)}({\cal G})\rig\Ga(\XX,\Dcm_{\XX}).$ D'autre part, comme 
l'algèbre $D^{(m)}(G)$ (resp. le faisceau $\Dm_{X}$) est séparé pour la topologie 
$p$-adique, on dispose d'injections canoniques $D^{(m)}(G)_K\hrig \what{D}^{(m)}({\cal G})_K$
(resp. $\Dm_{X_K}\hrig \Dcm_{X_K}$). 
Or $D^{(m)}(G)_K$ s'identifie à $U_K$ (resp. $\Dm_{X_K}$ à $\DD_{X_K}$). 
On dispose finalement du diagramme commutatif
$$\xymatrix { U_K^{op} \ar@{->}[r]^{Q_K}\ar@{^{(}->}[d]& \Ga(X_K,\DD_{X_K})\ar@{^{(}->}[d]\\
              \what{D}^{(m)}({\cal G})_K^{op} \ar@{->}[r]^{Q_m} & \Ga(\XX,\Dcm_{\XX,\Qr}), 
}$$
qui montre que $Q_m({Z_{K}}_+)=0$ et que $Q_m$ passe au quotient par ${Z_{K}}_+$ en une application 
toujours notée $Q_m$. On propose de montrer le
%
\begin{thm}\label{thm-glob_sections} \begin{enumerate} \item[(i)] On a un isomorphisme canonique 
               $$ Q_m\,\colon\, \what{D}^{(m)}({\cal G})_K^{op}/
{Z_{K}}_+\what{D}^{(m)}({\cal G})_K^{op} \sta{\sim}{\rig} \Ga(\XX,\Dcm_{\XX,\Qr}).$$
            \item[(ii)] On a un isomorphisme canonique 
               $$ Q\,\colon\, {D}^{\dagger}({\cal G})_K^{op}/
{Z_{K}}_+D^{\dagger}({\cal G})_K^{op} \sta{\sim}{\rig} \Ga(\XX,\Ddag_{\XX,\Qr}).$$
           \item[(iii)] L'idéal ${Z_{K}}_+$ est contenu dans le centre de 
         $\what{D}^{(m)}({\cal G})_K^{op}$ et de $D^{\dagger}({\cal G})_K^{op}$.
          \end{enumerate}
\end{thm} 
%
Le (ii) s'obtient par passage à la limite à partir de (i).
L'alinéa (i) sera démontré en ~\ref{dem_thm}.
Montrons (iii). Comme $D^{\dagger}({\cal G})_K$ est limite inductive des algèbres 
$\what{D}^{(m)}({\cal G})_K$, il suffit de montrer que ${Z_{K}}_+$ est dans le centre 
des algèbres $\what{D}^{(m)}({\cal G})_K$. Soient $\xi_1,\ldots,\xi_N$ 
une base de $Lie(G)$. L'algèbre $U_K$ est dense dans l'algèbre 
$\what{D}^{(m)}({\cal G})_K$ pour la topologie $p$-adique. Soit $t\in {Z_{K}}_+$, 
le commutateur $C_t$ est une application continue : $\what{D}^{(m)}({\cal G})_K\rig 
\what{D}^{(m)}({\cal G})_K$, qui s'annule sur $U_K$ et qui est donc nulle sur 
l'algèbre $\what{D}^{(m)}({\cal G})_K$. En particulier, les idéaux 
introduits dans l'énoncé $\what{D}^{(m)}({\cal G})_K{Z_{K}}_+$ et $D^{\dagger}({\cal G})_K{Z_{K}}_+$ sont bilatères.
%
\subsubsection{Enoncé du théorème dans le cas twisté}
Nous reprenons les notations de la sous-section précédente~\ref{enonce-thm_class}, et l'application 
$^t{}Q_m$ introduite en ~\ref{Qtmc} (resp. ~\ref{Qctm}), 
$^t{}Q_m $ : $\what{D}^{(m)}({\cal G})\rig\Ga(\XX,^t{}\Dcm_{\XX}).$ Dans le cas twisté, on dispose 
de l'analogue du diagramme commutatif précédent 
$$\xymatrix { U_K^{op} \ar@{->}[r]^{^t{}Q_K}\ar@{^{(}->}[d]& \Ga(X_K,^t{}\DD_{X_K})\ar@{^{(}->}[d]\\
              \what{D}^{(m)}({\cal G})_K^{op} \ar@{->}[r]^{^t{}Q_m} & \Ga(\XX,^t{}\Dcm_{\XX,\Qr}), 
}$$
qui montre que $Q_m(Ker\theta_K)=0$ et que $Q_m$ passe au quotient par $Ker\theta_K \,\what{D}^{(m)}({\cal G})_K^{op}$ 
en une application toujours notée $Q_m$. L'énoncé dans le cas twisté est 
%
\begin{thm}\label{thm-glob_sectionstw} \begin{enumerate} \item[(i)] On a un isomorphisme canonique 
               $$ Q_m\,\colon\, \what{D}^{(m)}({\cal G})_K^{op}/
 Ker\theta_K\,\what{D}^{(m)}({\cal G})_K^{op} \sta{\sim}{\rig} \Ga(\XX,^t{}\Dcm_{\XX,\Qr}).$$
            \item[(ii)] On a un isomorphisme canonique 
               $$ Q\,\colon\, {D}^{\dagger}({\cal G})_K^{op}/
Ker\theta_K \, D^{\dagger}({\cal G})_K^{op} \sta{\sim}{\rig} \Ga(\XX,^t{}\Ddag_{\XX,\Qr}).$$
                     \end{enumerate}
\end{thm} 
%
Observons comme précédemment que le (ii) s'obtient par passage à la limite sur $m$ à partir de (i).

\vspace{+2mm}
Nous montrons le (i) de ces théorèmes dans la suite de cet appendice. La démonstration repose,
en plus de toutes les constructions du corps de cet article, 
 sur les techniques utilisées en ~\cite{huy-beil_ber}.

\subsubsection{Démonstration du théorème}
\label{dem_thm}
Considérons, sur la variété de drapeaux de $X$, le faisceau de 
$\OO_X$-anneaux cohérent
$\AA^{(m)}_{X} = \OO_{X}\ot_V D^{(m)}(G)$ introduit en~\ref{prop-Am}. 
Etudions d'abord les propriétés cohomologiques des $\AA^{(m)}_{X}$-modules cohérents sur la variété de drapeaux. 
Soit $\MM$ un $\AA^{(m)}_{X}$-module cohérent. Nous avons la 
%
\begin{sousprop} \be \item[(i)] $\Ga(X,\AA^{(m)}_{X})=D^{(m)}(G)^{op}$ est une $V$-algèbre noetherienne.
                   \item[(ii)] Le module $\MM$ admet une résolution globale par 
   des modules du type $\AA^{(m)}_{X}(-r)^a$ avec $r\in\Ze$ et $a\in \Ne,$
          \item[(iii)] $\forall k \in \Ne$, $H^k(X,\MM)$ est un
$D^{(m)}(G)^{op}$-module de type fini.
\ee
\end{sousprop} 
%}}
\begin{proof}
 Comme $D^{(m)}(G)^{op}$ est un $V$-module libre, on a 
$\Ga(X,\AA^{(m)}_{X})=\Ga(X,\OO_X)\ot_V D^{(m)}(G)^{op}$ d'où le résultat 
puisque $\Ga(X,\OO_X)=V$ et que $D^{(m)}(G)^{op}$ est noetherien par ~\ref{grDm}. Le
 (ii) provient de 2.2.1 of \cite{huy-beil_ber} en remplaçant $\DD$ par
$\AA^{(m)}_{X}$. La démonstration de (ii) est aussi dans loc. cit. En effet, on montre (ii) 
par récurrence descendante en écrivant le longue suite exacte de cohomologie.
L' assertion est trivialement vraie pour $k=N+1$ car $H^{N+1}(X,\MM)=0$ puisque 
$\MM$ est limite inductive de faisceaux coherents sur $X$. De plus 
$D^{(m)}(G)^{op}=\Ga(X,\AA^{(m)}_{X})$ et
$$H^k(X,\AA^{(m)}_{X}(-r)^a)\simeq H^k(X,\OO_{X}(-r)^a)\ot_V D^{(m)}(G)^{op},$$
qui est un $D^{(m)}(G)^{op}$-module de type fini. Supposons que l'assertion soit vraie 
pour tout $\AA^{(m)}_{X}$-module cohérent et pour tout $l\geq k+1$. Soit $\MM$ un 
 $\AA^{(m)}_{X}$-module-cohérent.
Grâce à (ii), il existe
un $\AA^{(m)}_{X}$-module cohérent $\NN$, $r\in\Ze$, $a\in \Ne$ et une suite exacte courte
$$ 0 \rig \NN \rig \AA^{(m)}_{X}(-r)^a \rig \MM \rig 0.$$ En passant à la cohomologie, 
on trouve un complexe exact
$$ H^k(X,\AA^{(m)}_{X}(-r)^a) \rig H^k(X,\MM) \rig
H^{k+1}(X,\NN).$$
Comme $D^{(m)}(G)^{op}$ is noetherien, cela montre que $H^k(X,\MM)$ est un $D^{(m)}(G)^{op}$-module de type fini.
\end{proof}
%

On a un
morphisme filtré de $\OO_X$-anneaux $Q_{m,X}$ : $\AA^{(m)}_{X} \rig 
\Dm_X$ (resp. $^t{}Q_{m,X}$ : $\AA^{(m)}_{X} \rig  ^t{}\Dm_X$), qui est surjectif en passant aux gradués associés
 d'après (ii) de ~\ref{prop_grAm} (resp. ~\ref{grQtw}), ce qui montre par un argument classique que $Q_{m,X}$ est
surjectif. On obtient ainsi, grâce à la proposition précédente la 
%
\begin{sousprop} \be\item[(i)] $\Dm_X$ (resp. $^t{}\Dm_X$) est un $\AA^{(m)}_{X}$-module cohérent,
             \item[(ii)] $\Ga(X,\Dm_X)$ (resp. $\Ga(X,^t{}\Dm_X)$) est un $D^{(m)}(G)^{op}$-module de type fini.
              \ee
\end{sousprop} 
%

Rappelons maintenant le lemme suivant, dont la démonstration est laissée au lecteur.
\begin{surlem} Soient $A$ une $V$-algèbre noetherienne, $M$, $N$ deux $A$-modules de type fini,
  $u$ : $M \rig N$, une application $A$-linéaire, $\what{u}$ : $\what{M}\rig \what{N}$,
l'application induite par $u$ après complétion $\pi$-adique. 
 Supposons que  $u$ induise un isomorphisme après 
tensorisation par $\Qr$, $u\ot 1$ : $M_{\Qr}\rig N_{\Qr}$, alors $\what{u}\ot 1$ induit
un isomorphisme : $\what{M}_{\Qr}\rig \what{N}_{\Qr}$.
\end{surlem}
Considérons $Z_+={Z_{K}}_+\bigcap D^{(m)}(G)$, alors $Z_+\ot_V K={Z_{K}}_+$.
Nous appliquons ce lemme à $M=D^{(m)}(G)^{op}/D^{(m)}(G)^{op}Z_+ $, 
$N=\Ga(\XX,\DD^{(m)}_{X})$ qui est un $D^{(m)}(G)^{op}$-module de type fini par la proposition 
précédente et $Q_m$ : $D^{(m)}(G)^{op}/D^{(m)}(G)^{op}Z_+ \rig \Ga(\XX,\DD^{(m)}_{X})$. 

Le morphisme $Q_m \ot 1$ est le morphisme 
$D^{(0)}(G)_{\Qr}^{op}/ {Z_{K}}_+ D^{(0)}(G)_{\Qr}^{op} \rig \Ga(\XX,\DD_{X,\Qr})$ qui est un isomorphisme 
 grâce au résultat classique pour les $\DD$-modules algébriques en
car. $0$ rappelés en~\ref{rappels-Uclass}. La complétion dans un anneau noetherien 
et un foncteur exact de sorte que 
$\what{M}_{\Qr}\simeq \what{D}^{(m)}({\cal G}_K)^{op} / {Z_{K}}_+\what{D}^{(m)}({\cal G}_K)^{op}$. 
En outre, le complété $\pi$-adique de $N$ est $\Ga(\XX,\Dcm_{\XX})$ d'après 3.2.6 de \cite{EGA1}. 
On déduit alors du lemme précédent que le complété de $Q_m$ : 
$\what{D}^{(m)}({\cal G}_K)^{op} / {Z_{K}}_+\what{D}^{(m)}({\cal G}_K)^{op} \rig 
\Ga(\XX,\Dcm_{\XX,\Qr}),$ est un isomorphisme. Le (ii) du théorème s'obtient à partir du 
(i) par passage à la limite inductive sur $m$, ce qui achève la démonstration du théorème ~\ref{thm-glob_sections} 
dans le cas non twisté.

Pour avoir le théorème dans le cas twisté, on pose $Ker\theta=Ker\theta_K \bigcap D^{(m)}(G)$, 
$M=D^{(m)}(G)^{op}/D^{(m)}(G)^{op}Ker\theta$. Nous appliquons alors le lemme précédent 
à $M$, $N=\Ga(\XX,^t{}\DD^{(m)}_{X})$ et $^t{}Q_m$ : $M \rig
 N$. Grâce au théorème de Beilinson-Bernstein pour le cas twisté rappelé en 
~\ref{rappels-Uclass}, le morphisme $^t{}Q_m\ot 1$ est un isomorphisme. De plus, 
 $\what{M}_{\Qr}\simeq \what{D}^{(m)}({\cal G}_K)^{op} / Ker\theta_K\what{D}^{(m)}({\cal G}_K)^{op}$ et
le complété $\pi$-adique de $N$ est $\Ga(\XX,^t{}\Dcm_{\XX})$. En appliquant le lemme précédent, on voit donc 
que l'on a un isomorphisme $\what{D}^{(m)}({\cal G})_K^{op}/
 Ker\theta_K\,\what{D}^{(m)}({\cal G})_K^{op} \sta{\sim}{\rig} \Ga(\XX,^t{}\Dcm_{\XX,\Qr}),$
ce qui achève la démonstration du théorème.
